# Supplementary material for: SHOVIR: A Benchmark for Evaluating Vision Shortcut Learning in Radiology Report Generation
Source: arXiv:2606.30201 source file (2026-10-18)
Supplement: Supplementary file 1 [file supplementary_v1.tex]

%s WACV 2027 Paper Template
% based on the ICCV 2025 template (https://media.eventhosts.cc/Conferences/ICCV2025/ICCV2025-Author-Kit-Feb.zip) with
% WACV-specific details (e.g., 2 tracks) from the WACV 2025 template (https://www.dropbox.com/scl/fi/su44zgdhrzik26p2xu37k/WACV-2025-Author-Kit-Template.zip?rlkey=5qcfimjhxnmx3wlyk7yhk8wg7&dl=0)

\documentclass[10pt,twocolumn,letterpaper]{article}

%%%%%%%%% PAPER TYPE  - PLEASE UPDATE FOR FINAL VERSION
%   \usepackage[review,algorithms]{wacv}      % To produce the REVIEW version for the algorithms track
% \usepackage[review,applications]{wacv}      % To produce the REVIEW version for the applications track
\usepackage[review,datasets]{wacv}      % To produce the REVIEW version for the datasets track

\definecolor{colorDOCO}{HTML}{365F88}
\definecolor{colorMIMIC}{HTML}{1C7A30}
\definecolor{colorPadChest}{HTML}{2244AA}
\definecolor{colorOCO}{HTML}{BF525F}

% Shading
\definecolor{noisebg}{HTML}{EDF2F7}   % light blue-gray for noise columns
\definecolor{deltabg}{HTML}{E2E0EC}   % light purple-gray for delta columns

  % noise cell
  % delta cell

\usepackage{color}

\usepackage{colortbl}
\definecolor{deltabg}{gray}{0.92}

\newcommand{\mycomment}[1]{}
\newcolumntype{L}[1]{>{\raggedright\arraybackslash}p{#1}}
\newcolumntype{C}[1]{>{\centering\arraybackslash}p{#1}}
\usepackage[accsupp]{axessibility}

% ---------------------------------------------------------------
% TODO FINAL: Comment out the following line for the camera-ready version
%\usepackage[pagebackref,breaklinks,colorlinks,citecolor=eccvblue]{hyperref}
% TODO FINAL: Un-comment the following line for the camera-ready version

% Support for ORCID icon
\usepackage{orcidlink}

% Import additional packages in the preamble file, before hyperref
\input{preamble}

% It is strongly recommended to use hyperref, especially for the review version.
% hyperref with option pagebackref eases the reviewers' job.
% Please disable hyperref *only* if you encounter grave issues, 
% e.g. with the file validation for the camera-ready version.
%
% If you comment hyperref and then uncomment it, you should delete *.aux before re-running LaTeX.
% (Or just hit 'q' on the first LaTeX run, let it finish, and you should be clear).
\definecolor{wacvblue}{rgb}{0.21,0.49,0.74}
%\usepackage[pagebackref,breaklinks,colorlinks,allcolors=wacvblue]{hyperref}

%%%%%%%%% PAPER ID  - PLEASE UPDATE
 % *** Enter the WACV Paper ID here

\begin{document}

\title{\textbf{Supplementary Material}\\
       \large \textsc{ShoViR}: A Benchmark for Evaluating \\ Vision Shortcut Learning in \\ Radiology Report Generation}
\maketitle

\section{Datasets Curation }
\label{sec:data_supp}
This section details the mappings that unify the ChestImaGenome and PadChest-GR annotation vocabularies into the CheXpert label space, complementing Section~3.1 of the main paper.
s\subsection{MIMIC-CXR~\cite{johnson2019mimic}.} 

\noindent\textbf{Dataset overview.}
MIMIC-CXR is among the most widely adopted chest radiograph corpora, comprising 377,110 images from 227,827 studies, each paired with a free-text radiology report and image-level CheXpert labels.
We build on the official test split, which contains \textbf{3,858 images}.
To obtain spatial annotations, we incorporate ChestImaGenome~\cite{wu2021chest}, which extends a subset of MIMIC-CXR with structured bounding boxes associating clinical findings with anatomical regions.
Each annotation consists of an anatomical region label, one or more free-text attribute strings describing the radiological observation, and a bounding box $[x_1, y_1, x_2, y_2]$ localising the finding in the image.
The attribute vocabulary comprises 162 unique strings drawn from a clinical ontology that does not align one-to-one with the 14 CheXpert classes, as overlapping radiological concepts may be interpreted and labelled differently even for the same image.

\noindent\textbf{Preprocessing pipeline.}
Constructing a CheXpert-aligned evaluation set from the raw ImaGenome annotations involves four successive stages.

\begin{table*}[!h]
\centering
\caption{Complete ImaGenome-to-CheXpert attribute mapping. Attributes 
         marked with $\dagger$ are assigned to more than one class.}
\label{tab:mapping_full}
\footnotesize
\setlength{\tabcolsep}{4pt}
\fontsize{7pt}{7pt}\selectfont
\resizebox{\textwidth}{!}{
\begin{tabular}{L{3.2cm} L{7.8cm}}

\toprule
\textbf{CheXpert Class} & \textbf{ImaGenome Attribute Strings} \\
\midrule
Enlarged Cardiomediastinum 
  & mediastinal widening/enlargement, widened mediastinum,
    enlarged cardiac silhouette \\
\midrule
Cardiomegaly               
  & cardiomegaly, cardiac enlargement \\
\midrule
Lung Opacity               
  & lung opacity, opacity, airspace opacity/disease,
    hazy opacity$^{\dagger}$, infiltrate/infiltration, breast/nipple shadows \\
\midrule
Lung Lesion                
  & lung lesion/mass, nodule/mass, pulmonary nodule/mass,
    calcified nodule/granuloma, granuloma, lung cancer \\
\midrule
Edema                      
  & pulmonary edema, edema, vascular/pulmonary vascular congestion,
    interstitial/alveolar edema, fluid overload (heart failure),
    vascular redistribution, cephalization, interstitial thickening/prominence,
    vascular fullness, perihilar haze, hazy opacity$^{\dagger}$ \\
\midrule
Consolidation              
  & consolidation, consolidative (opacity), lobar consolidation \\
\midrule
Pneumonia                  
  & pneumonia \\
\midrule
Atelectasis                
  & atelectasis, atelectatic, collapse, lobar/lung/lobar-segmental collapse,
    linear/patchy/subsegmental/bibasilar/basilar/band-like/platelike/discoid
    atelectasis, volume loss \\
\midrule
Pneumothorax               
  & pneumothorax, ptx, hydropneumothorax, tension pneumothorax \\
\midrule
Pleural Effusion           
  & pleural effusion, effusion, pleural fluid, hydrothorax,
    layering/loculated effusion, costophrenic angle blunting \\
\midrule
Pleural Other              
  & pleural thickening/scarring/plaque/calcification/reaction,
    pleural-parenchymal scarring, apical pleural thickening/scarring \\
\midrule
Fracture                   
  & fracture, rib/clavicular/vertebral/sternal/scapular/spinal fracture,
    compression fracture, healing/healed/old/acute fracture \\
\midrule
Support Devices            
  & \textit{Tubes:} ET/tracheostomy/NG/OG/feeding/enteric/drainage
    tube, dobhoff, drain.
    \textit{Lines:} central venous catheter/line, PICC, swan-ganz,
    pulmonary artery/dialysis catheter, port-a-cath, arterial/venous line.
    \textit{Cardiac:} pacemaker, pacer, AICD, ICD, defibrillator,
    pacemaker lead(s), cardiac leads/wires.
    \textit{Surgical:} IABP, LVAD, ECMO, clips, staples,
    prosthetic valve, CABG, stent, hardware, sternotomy wires. \\
\bottomrule
\end{tabular}
}
\end{table*}

\begin{enumerate}
    \item \textbf{Spatial filtering.}
    Of the 3,858 test-split images, only those with at least one ImaGenome bounding box are eligible.
    This stage removes \textbf{1,397 images} lacking spatial annotations and a further \textbf{232 images} whose sole positive CheXpert label is \textit{No Finding}, which carries no associated bounding box, producing \textbf{2,229 candidate images} with both image-level labels and region-level annotations.

    \item \textbf{Label mapping to CheXpert classes.}
    The ImaGenome attribute vocabulary does not conform to the CheXpert convention.
    To reconcile the two label spaces, we define a rule-based mapping:
    \[
        \mathcal{M}: \mathcal{A} \;\longrightarrow\; 2^{\mathcal{C}},
    \]
    where $\mathcal{A}$ denotes the set of ImaGenome attribute strings and $\mathcal{C}$ the 13 localisable CheXpert classes (\textit{No Finding} is excluded as it carries no spatial grounding).
    We leveraged Claude Opus~4.6~\cite{anthropic2025claude} to draft an initial assignment of each attribute to one or more CheXpert classes following standard radiological nomenclature; all assignments were subsequently validated through the verification stages described below.
    The full mapping is reported in Table~\ref{tab:mapping_full}.

    \item \textbf{Cross-source validation.}
    Since the CheXpert labels and ImaGenome attributes originate from independent annotation processes, we perform a consistency verification.
    For every image-class pair in the test split, the original CheXpert labels are compared against those inferred from the mapped ImaGenome attributes, yielding an F1 of $\mathbf{0.935}$, confirming strong concordance between the two sources.

    \item \textbf{True-positive filtering.}
    To prevent noisy labels from undermining the occlusion analysis, we enforce a strict confirmation criterion: an image is kept only if \emph{every} positive CheXpert class is supported by at least one affirmed ImaGenome attribute.
    Formally, an image $\mathcal{I}$ with positive label set $\mathcal{D}_{\mathcal{I}} \subseteq \mathcal{C}$ passes if and only if:
    \[
        \forall\, c \in \mathcal{D}_{\mathcal{I}},\;\;
        \exists\, a \in \mathcal{A}(\mathcal{I}) \;\text{s.t.}\;
        c \in \mathcal{M}(a),
    \]
    where $\mathcal{A}(\mathcal{I})$ denotes the set of affirmed ImaGenome attributes for image $\mathcal{I}$.
    This stage removes \textbf{69 images}, leaving \textbf{2,160 images}.
\end{enumerate}

\noindent\textbf{Final dataset.}
The final subset contains \textbf{2,160 unique images}, each accompanied by a radiology report, multi-label annotations across the 13 localisable CheXpert classes, and region-level bounding boxes linking each positive finding to its anatomical location.

\subsection{PadChest-GR~\cite{de2025padchest}}

\noindent\textbf{Dataset overview.}
PadChest-GR is a grounded radiology report dataset comprising \textbf{4,555 studies}, each consisting of a frontal chest X-ray paired with a structured set of radiological findings. 
Unlike standard classification datasets, each finding is represented as a triplet: (i) a free-text sentence in both English and Spanish describing the radiological observation, (ii) one or more normalised bounding boxes $[x_1, y_1, x_2, y_2] \in [0,1]^4$ localizing the finding in the image, and (iii) one or more categorical labels drawn from a vocabulary of 154 unique finding types. 
An additional \texttt{progression} field links each finding to a prior study when available, enabling longitudinal comparisons. Table~\ref{tab:padchest_schema} describes the complete schema of a raw dataset entry.

\begin{table*}[h]
\centering
\caption{Schema of a single study entry in the raw PadChest-GR JSON file \texttt{grounded\_reports\_20240819.json}. 
Each study contains a list of \texttt{findings}, each of which may carry bounding-box annotations and categorical labels.}
\label{tab:padchest_schema}
\small
\fontsize{7pt}{7pt}\selectfont
\resizebox{\textwidth}{!}{
\begin{tabular}{llp{7cm}}
\toprule
\textbf{Field} & \textbf{Type} & \textbf{Description} \\
\midrule
\multicolumn{3}{l}{\textit{Study-level fields}} \\
\midrule
\texttt{StudyID}          & string        & Unique alphanumeric study identifier \\
\texttt{ImageID}          & string        & Filename of the associated X-ray image (\texttt{.png}) \\
\texttt{PreviousStudyID}  & string / null & Study ID of the chronological predecessor, if available \\
\texttt{PreviousImageID}  & string / null & Image filename of the chronological predecessor \\
\midrule
\multicolumn{3}{l}{\textit{Finding-level fields} (repeated for each finding within a study)} \\
\midrule
\texttt{sentence\_en}     & string        & Radiological finding sentence in English \\
\texttt{sentence\_es}     & string        & Radiological finding sentence in Spanish \\
\texttt{abnormal}         & bool          & Whether the finding describes a radiological abnormality \\
\texttt{boxes}            & list of $[x_1,y_1,x_2,y_2]$ & Primary normalised bounding boxes (may be empty) \\
\texttt{extra\_boxes}     & list of $[x_1,y_1,x_2,y_2]$ & Secondary/alternative bounding boxes (may be empty) \\
\texttt{labels}           & list of strings & Categorical finding labels from the PadChest vocabulary (154 types) \\
\texttt{locations}        & list of strings & Free-text anatomical location descriptors \\
\texttt{progression}      & string / null & Change descriptor relative to the prior study (\textit{e.g.,} ``improved'', ``stable'') \\
\bottomrule
\end{tabular}
}
\end{table*}

\noindent\textbf{Preprocessing pipeline.}
Obtaining a clean, CheXpert-aligned evaluation set from the raw PadChest-GR data requires a multi-step filtering and mapping pipeline. 
The quantitative effect of each step is summarized in Table~\ref{tab:padchest_funnel}.

\begin{table*}[!h]
\centering
\caption{Quantitative effect of each preprocessing step on the PadChest-GR dataset.}
\label{tab:padchest_funnel}
\small
\fontsize{10pt}{8pt}\selectfont
\resizebox{\textwidth}{!}{
\begin{tabular}{lrrl}
\toprule
\textbf{Processing step} & \textbf{Studies / Images} & \textbf{Box annotations} & \textbf{Notes} \\
\midrule
Raw dataset                                   & 4,555  & 7,733 & 154 finding label types \\
After spatial filtering                        & 3,008  & 7,733 & 66.0\% of studies retained \\
After label mapping (69 / 154 labels)         & 3,008  & 3,015 & 43\% of annotated mentions \\
After CheXbert validation                      & ---    & 2,001 & 1,014 annotations discarded (33.6\%) \\
After minimum class-size filter ($\geq 40$)   & 1,390  & 1,997 & 3 classes removed; 9 retained \\
\bottomrule
\end{tabular}
}
\end{table*}

\begin{enumerate}

    \item \textbf{Spatial filtering.}
    Of the 4,555 raw studies, only those containing at least one annotated bounding box are retained for evaluation. 
    Across all studies, 10,479 finding sentences are recorded, of which 6,217 carry at least one bounding box, corresponding to 7,733 individual box annotations in total. 
    At the study level, \textbf{3,008 studies} (66.0\%) contain at least one grounded finding; the remaining 1,547 studies (34.0\%) consist exclusively of box-free findings (\textit{e.g.}, negative reports or findings that cannot be localised) and are discarded.

    \item \textbf{Label mapping to CheXpert classes.}
    PadChest-GR uses a domain-specific vocabulary of 154 unique finding labels that does not conform to the CheXpert convention. 
    To align the dataset with a unified label space, we derive a deterministic rule-based mapping:
    \[
        \mathcal{M}: \mathcal{L} \;\longrightarrow\; 2^{\mathcal{C}},
    \]
    where $\mathcal{L}$ denotes the set of PadChest-GR label strings and $\mathcal{C}$ the 13 localizable CheXpert classes (\textit{No Finding} is excluded as it carries no spatial grounding).
    A static lookup table maps 69 of the 154 labels to one or more CheXpert categories. We leveraged Claude Opus~4.6~\cite{anthropic2025claude} to propose an initial assignment of each label according to standard radiological nomenclature; all assignments were subsequently reviewed and corrected by the authors.
    The remaining 85 labels have no unambiguous correspondence to any CheXpert class and are excluded together with their associated bounding boxes. 
    Polysemous labels may receive multiple target classes (\textit{e.g.}, \textit{alveolar pattern} maps to both Lung Opacity and Consolidation). 
    After this step, \textbf{3,015 box-level annotations} remain as candidates for evaluation. 
    The full mapping is summarized in Table~\ref{tab:padchest_mapping_full}.

    \item \textbf{CheXbert consistency validation.}
    Label mapping is inherently noisy: a PadChest finding label may be mapped to a CheXpert class that is not supported by the accompanying radiological sentence. To mitigate this, each mapped bounding box is cross-validated against the output of CheXbert~\cite{smit2020chexbert}, a BERT-based classifier fine-tuned for CheXpert label extraction, applied to the \texttt{sentence\_en} field associated with the box. If the CheXbert-predicted class disagrees with the mapped CheXpert label, the annotation is discarded. Formally, a box $b$ with mapped label $c \in \mathcal{C}$ is retained if and only if:
    \[
        \text{CheXbert}(\texttt{sentence\_en}(b)) \ni c.
    \]
    This step discards \textbf{1,014 annotations} (33.6\%), leaving \textbf{2,001 verified box-level annotations}. The filtering is conservative by design: it prioritises annotation precision over recall, accepting reduced coverage in exchange for higher label fidelity.

    \item \textbf{Minimum class-size filtering.}
    To ensure reliable per-class evaluation, classes with fewer than \textbf{40 annotated images} after the preceding steps are excluded. 
    Three CheXpert categories fall below this threshold: \textit{Edema} (3 images), \textit{Pneumothorax} (8 images), and \textit{Enlarged Cardiomediastinum} (38 images). 
    Their removal yields a final set of \textbf{9 retained classes}.

\end{enumerate}

\noindent\textbf{Final dataset.}
The resulting evaluation set comprises 1,390 unique images with 1,997 annotated bounding box regions distributed across 9 CheXpert categories. 
Each image is assigned to one or more class-specific files, one per retained category, allowing per-class evaluation. 
Note that the total count of (image, class) pairs across files (1,903) exceeds the number of unique images (1,390) because a single image may contain findings belonging to multiple categories. 

\begin{table*}[h]
\centering
\caption{Complete PadChest-GR to CheXpert label mapping. }
\label{tab:padchest_mapping_full}
\footnotesize
\setlength{\tabcolsep}{4pt}
\fontsize{7pt}{7pt}\selectfont
\resizebox{\textwidth}{!}{
\begin{tabular}{L{3.2cm} L{7.8cm}}
\toprule
\textbf{CheXpert Class} & \textbf{PadChest-GR Label Categories} \\
\midrule
Enlarged Cardiomediastinum
  & mediastinal enlargement, superior mediastinal enlargement,
    mediastinic lipomatosis, aortic button enlargement \\
\midrule
Cardiomegaly
  & cardiomegaly \\
\midrule
Lung Opacity
  & increased density, infiltrates, interstitial pattern,
    reticular interstitial pattern, reticulonodular interstitial pattern,
    miliary opacities, air bronchogram \\
\midrule
Lung Lesion
  & nodule, multiple nodules, mass, pulmonary mass,
    calcified granuloma, granuloma, cavitation, cyst, abscess \\
\midrule
Edema
  & hilar congestion, kerley lines, ground glass pattern \\
\midrule
Consolidation
  & consolidation, alveolar pattern \\
\midrule
Pneumonia
  & pneumonia \\
\midrule
Atelectasis
  & atelectasis, atelectasis basal, laminar atelectasis,
    lobar atelectasis, segmental atelectasis, total atelectasis \\
\midrule
Pneumothorax
  & pneumothorax, hydropneumothorax \\
\midrule
Pleural Effusion
  & pleural effusion, loculated pleural effusion,
    loculated fissural effusion \\
\midrule
Pleural Other
  & pleural thickening, apical pleural thickening,
    calcified pleural thickening, calcified pleural plaques,
    fissure thickening, major fissure thickening,
    minor fissure thickening, costophrenic angle blunting, pleural mass \\
\midrule
Fracture
  & fracture, callus rib fracture, rib fracture, clavicle fracture,
    humeral fracture, vertebral fracture, vertebral compression,
    vertebral anterior compression \\
\midrule
Support Devices
  & \textit{Pacing:} pacemaker, dual chamber device, single chamber device.
    \textit{Tubes:} NSG tube, endotracheal tube, tracheostomy tube,
    chest drain tube, gastrostomy tube, ventriculoperitoneal drain tube.
    \textit{Lines:} central venous catheter, central venous catheter via
    jugular vein, central venous catheter via subclavian vein,
    reservoir central venous catheter, catheter.
    \textit{Other:} electrical device. \\

\bottomrule
\end{tabular}
}
\end{table*}

\subsection{Radiologist Validation of the Pathology Mapping}
\label{sec:radiologist_validation}
To assess the reliability of the label mapping used in our annotation pipeline, we conducted a systematic radiologist validation on both datasets.
For each of the 13 CheXpert pathology classes present in MIMIC-CXR and the 9 classes present in PadChest-GR, we randomly sampled 5 cases per class, yielding 65 and 45 validation cases, respectively. For each case, a radiologist was presented with: (i)~the chest radiograph with the annotated bounding box overlaid on the finding region of interest, (ii)~the original textual finding from the dataset annotation, and (iii)~the full radiology report. The radiologist was then asked to independently assign the most appropriate CheXpert label from the candidate set, without prior knowledge of the automated mapping.
Agreement between the radiologist's independent classification and our automated mapping was 100\% on both MIMIC-CXR and PadChest-GR.
In addition, the radiologist reviewed the complete rule-based mapping tables (Table~\ref{tab:mapping_full} and Table~\ref{tab:padchest_mapping_full}) and confirmed that every CheXpert assignment is clinically appropriate.
These results provide strong evidence that the proposed mapping faithfully reflects expert radiological judgment across both datasets.

\section{Occlusion Protocol Details}
\label{sec:occlusion_supp}
This section details the mathematical formulation of the matched correlated noise used in both the Full Noise Image and Disease-Level Occlusion settings, and validates the choice of occluder type through a controlled ablation.

\subsection{Noise Formulation}
\label{sec:noise_formulation}
We describe here the mathematical formulation of the matched correlated noise used in both the \textit{Full Noise Image} and \textit{Disease-Level Occlusion} settings.

\noindent\textbf{Full Noise Image.} 
For each image~$\mathcal{I}$ with pixel values~$x$, we first compute robust statistics from the central intensity range:

$$\mu_{\mathcal{I}} = \mathrm{mean}(x_{[1\%,\,99\%]}), \qquad \sigma_{\mathcal{I}} = \mathrm{std}(x_{[1\%,\,99\%]})$$

where~$x_{[1\%,\,99\%]}$ denotes pixel values between the 1st and 99th percentiles, trimmed to reduce the influence of outliers. We then generate the full noise image as:

$$\mathcal{I}_{\mathrm{noise}} = G_{\sigma_s} * \mathcal{N}(\mu_{\mathcal{I}},\, \sigma_{\mathcal{I}}^2)$$

where~$\mathcal{N}(\mu_{\mathcal{I}},\, \sigma_{\mathcal{I}}^2)$ denotes pixel-wise i.i.d.\ Gaussian noise with matched moments,~$*$ denotes 2D spatial convolution, and~$G_{\sigma_s}$ is a Gaussian smoothing kernel:

$$G_{\sigma_s}(x, y) = \frac{1}{2\pi\sigma_s^2} \exp\!\left(-\frac{x^2 + y^2}{2\sigma_s^2}\right)$$

with~$\sigma_s{=}2.0$\,px, introducing mild local spatial correlations that mimic the coarse texture of the original radiograph without preserving any anatomical or pathological content.

\noindent\textbf{Disease-Level Occlusion.} 
For the disease-level conditions (RO, OCO, DOCO), noise is generated with the same procedure and restricted to the target bounding boxes. 
Given an occlusion strength~$p \in \{0, 0.2, 0.4, 0.6, 0.8, 1.0\}$, the pixel values within each target box~$b$ are computed as:

$$\mathcal{I}_{\mathrm{occ}}(b) = (1 - p) \cdot \mathcal{I}(b) + p \cdot \mathcal{I}_{\mathrm{noise}}(b)$$

where~$\mathcal{I}(b)$ denotes the original pixel values within~$b$ and~$\mathcal{I}_{\mathrm{noise}}(b)$ the corresponding noise patch. The parameter~$p$ linearly interpolates between the original content ($p{=}0$, Baseline) and full noise replacement ($p{=}1.0$). To prevent the sharp rectangular boundary of the noise patch from acting as a detectable artifact, we apply a feathered edge by multiplying~$p$ with a smooth falloff mask~$\alpha(x,y)$ that decays from 1 at the box interior to 0 at the boundary:

$$\mathcal{I}_{\mathrm{occ}}(x,y) = (1 - p \cdot \alpha(x,y)) \cdot \mathcal{I}(x,y) + p \cdot \alpha(x,y) \cdot \mathcal{I}_{\mathrm{noise}}(x,y)$$

This ensures a gradual transition between occluded and clean regions, so that models respond to the removal of diagnostic content rather than to the presence of an obvious rectangular patch.

\subsection{Sensitivity to occluder type.}
A natural concern is whether the specific noise pattern used for occlusion could itself bias model predictions, independently of the diagnostic content being removed.
The \textsc{RO} condition already provides a first control: since noise is applied outside both the target and co-disease regions, any performance drop under \textsc{OCO} or \textsc{DOCO} beyond the \textsc{RO} baseline can be attributed to the removal of diagnostically relevant content rather than to encoder sensitivity to the fill pattern.

To further validate this finding, we compare six alternative occluder types against our matched correlated noise (MCN) under \textsc{RO} at $p{=}100\%$ on MIMIC-CXR.
We select CXRMate as the testbed because it exhibits the highest $\mu$-F1 sensitivity to random occlusion among all evaluated models (cf.\ Figure~2 in the main paper), making it the most conservative setting for detecting occluder-induced artifacts.
The six alternatives span a range of statistical and perceptual properties:
uniform uncorrelated noise (UUN), which samples pixel values uniformly at random;
healthy-tissue patch (HTP), which replaces the occluded region with a patch from a radiograph without pathological findings;
matched uncorrelated noise (MUN), which preserves the per-image mean and standard deviation but lacks spatial correlation;
dataset mean fill (DMF), which replaces the region with the global mean pixel value computed across the dataset;
patch mean fill (PMF), which uses the local mean of the occluded region itself;
and Gaussian blur (GB), which applies heavy spatial blurring to the original content within the bounding box.

Table~\ref{tab:occluder_ablation} reports the results.
All seven occluder variants yield $\mu$-F1 scores within a narrow 0.8 percentage-point range of one another (0.649--0.657), and the strongest occluder (UUN) reduces $\mu$-F1 by at most 4.0 percentage points relative to the unoccluded baseline (0.689).
Notably, our MCN approach ($\mu$-F1 = 0.655) ranks among the least disruptive occluders, while, unlike GB and PMF, it derives no information from the content of the occluded region itself.
This property is desirable: an occluder that retains local statistics from the target area could inadvertently preserve low-level cues that models exploit, weakening the diagnostic validity of the occlusion.
These results confirm that the choice of fill pattern has a negligible effect on model predictions under \textsc{RO}, and that the performance drops observed under \textsc{OCO} and \textsc{DOCO} in our main experiments reflect genuine dependence on diagnostic visual evidence rather than sensitivity to a particular noise texture.

\begin{table*}[t]
\centering
\caption{Occluder-type ablation under \textsc{RO} at $p{=}100\%$ for CXRMate on MIMIC-CXR.
The unoccluded baseline (Base.) is shown for reference.}
\label{tab:occluder_ablation}
\fontsize{7pt}{8pt}\selectfont
\setlength{\tabcolsep}{4pt}
\renewcommand{\arraystretch}{1.10}
\begin{tabular}{L{1.8cm} C{1.0cm} C{1.0cm} C{1.0cm} C{1.0cm} C{1.0cm} C{1.0cm} C{1.4cm} C{1.0cm}}
\toprule
 & UUN & HTP & MUN & DMF & PMF & GB & MCN (ours) & Base. \\
\midrule
$\mu$-F1 & 0.649 & 0.650 & 0.652 & 0.654 & 0.656 & 0.657 & 0.655 & 0.689 \\
\bottomrule
\end{tabular}
\end{table*}

\section{Vision Language Models}

We provide detailed descriptions of the nine VLMs evaluated in this work, as listed in \Cref{tab:architectures}. 

\begin{table*}[!h]
\centering
\caption{Architecture summary of the evaluated VLMs. We report the vision encoder, multimodal adapter, language decoder, and parameters count for each model.}
\label{tab:architectures}
\resizebox{0.8\textwidth}{!}{%
\begin{tabular}{lllll}
\toprule
\textbf{Model} & \textbf{Vision Encoder} & \textbf{Adapter} & \textbf{Language Decoder} & \textbf{$\sim$Params} \\
\midrule
CheXagent-2~\cite{chen2024chexagent}       &  SigLIP~\cite{zhai2023sigmoid}        & MLP       & Phi-2~\cite{javaheripi2023phi}                    & 3B  \\
CXRMate~\cite{nicolson2024health}      & UniFormer~\cite{li2023uniformer}               & MLP              & LLaMA-style~\cite{touvron2023llama}       & 0.2B \\
Libra-v1~\cite{zhang2025libra}           & RAD-DINO~\cite{perez2025exploring}             & TAC~\cite{zhang2025libra}                             & Meditron~\cite{chen2023meditron}                   & 7B  \\
LLaVA-Rad~\cite{chaves2024llavarad}       & BiomedCLIP-CXR~\cite{chaves2024llavarad}               & MLP                 & Vicuna~\cite{chiang2023vicuna}         & 7B  \\
MAIRA-2~\cite{bannur2024maira2}         & RAD-DINO~\cite{perez2025exploring}             & MLP                   & Vicuna~\cite{chiang2023vicuna}                      & 7B  \\
MedGemma~\cite{sellergren2025medgemma}   & MedSigLIP~\cite{sellergren2025medgemma}     & Gemma~3 adapter~\cite{gemmateam2025gemma3technicalreport}                  & Gemma~3~\cite{gemmateam2025gemma3technicalreport}                        & 4B  \\
RaDialog~\cite{pellegrini2023radialog}        & BioViL-T~\cite{bannur2023learning}                     & Alignment Module~\cite{pellegrini2023radialog}         & Vicuna~\cite{chiang2023vicuna}                     & 7B  \\
NV-Reason-CXR~\cite{myronenko2025reasoning}   & Qwen ViT~\cite{bai2025qwen25vltechnicalreport}      & MLP            & Qwen2.5~\cite{bai2025qwen25vltechnicalreport}                 & 3B  \\
\bottomrule
\end{tabular}%
}
\end{table*}
\subsection{Architectures}

\noindent\emph{CheXagent-2}~\cite{chen2024chexagent} is a vision-language foundation model built on a 2.7B-parameter Phi-2 language backbone~\cite{javaheripi2023phi}, trained through a three-stage pipeline: clinical LLM pre-training, CXR vision encoder training, and vision-language instruction tuning on CheXinstruct~\cite{chen2024chexagent}, a dataset curated from 28 publicly available CXR datasets.

\noindent\emph{CXRMate}~\cite{nicolson2024health} is a multimodal language model pairing a CXR image encoder with a Llama-based decoder, trained via Entropy-Augmented Self-Critical Sequence Training (EAST), which extends SCST~\cite{rennie2017self} with entropy regularisation to prevent policy collapse onto common phrases, using RadGraph-F1~\cite{jain2021radgraph} as the reward signal.

\noindent\emph{Libra}~\cite{zhang2025libra} is a temporal-aware model that explicitly captures longitudinal changes between current and prior chest X-rays through a Temporal Alignment Connector, which fuses multi-layer features from a radiology-specific RAD-DINO encoder before feeding them into a Meditron-7B~\cite{bosselut2024meditron} language backbone.

\noindent\emph{LLaVA-Rad}~\cite{chaves2024llavarad} follows the LLaVA-style~\cite{liu2024visual} recipe of coupling a vision encoder with a lightweight adapter and a 7B-class decoder, with the key specialization of using BiomedCLIP-CXR~\cite{chaves2024llavarad} as the image encoder to improve clinical correctness on chest radiographs.

\noindent\emph{MAIRA-2}~\cite{bannur2024maira2} adopts the LLaVA-1.5 architecture~\cite{liu2024visual} and couples RAD-DINO~\cite{perez2025exploring} with a Vicuna-7B decoder. 
It further leverages large-scale data engineering, including synthetic augmentation, to improve report quality and robustness.

\noindent\emph{MedGemma}~\cite{sellergren2025medgemma} is Google's open medical multimodal family built on Gemma~3, using MedSigLIP as a medical image encoder shared across model sizes. 
We evaluate the 4B variant, which pairs a SigLIP-400M-class vision encoder~\cite{zhai2023sigmoid} with a Gemma~3 language backbone.

\noindent\emph{RaDialog}~\cite{pellegrini2023radialog} frames report generation as part of interactive radiology assistance, integrating visual features from a BioViL-T encoder~\cite{bannur2023learning} and structured pathology findings into a Vicuna-7B language model~\cite{chiang2023vicuna} through an alignment module and parameter-efficient LoRA tuning~\cite{hu2022lora}.

\noindent\emph{NV-Reason-CXR}~\cite{myronenko2025reasoning} is a 3B-parameter reasoning-focused VLM obtained by fine-tuning Qwen2.5-VL-3B~\cite{bai2025qwen25vltechnicalreport}  through supervised fine-tuning on expert radiologist reasoning data, followed by Group Relative Policy Optimization with verifiable rewards~\cite{shao2024deepseekmath} over CheXpert abnormalities, to produce chain-of-thought diagnostic rationales.

Table~\ref{tab:model_overview} lists the nine evaluated models with their
HuggingFace Hub identifiers, numerical precision, and the Python virtual
environment used for inference.
Because of irreconcilable dependency conflicts between model families, five
separate environments are maintained.

\begin{table*}[ht]
\centering
\caption{Model overview. HF~ID = HuggingFace Hub model identifier.}
\label{tab:model_overview}
\fontsize{11pt}{12pt}\selectfont
\setlength{\tabcolsep}{4pt}
\begin{tabular}{L{3cm} L{12.0cm}}
\toprule
\textbf{Model} & \textbf{HuggingFace Hub ID} \\
\midrule
MedGemma      & \href{https://huggingface.co/google/medgemma-1.5-4b-it}{\nolinkurl{google/medgemma-1.5-4b-it}} \\
MAIRA-2       & \href{https://huggingface.co/microsoft/maira-2}{\nolinkurl{microsoft/maira-2}} \\
CXRMate       & \href{https://huggingface.co/aehrc/cxrmate-rrg24}{\nolinkurl{aehrc/cxrmate-rrg24}} \\
NV-Reason-CXR & \href{https://huggingface.co/nvidia/NV-Reason-CXR-3B}{\nolinkurl{nvidia/NV-Reason-CXR-3B}} \\
LIBRA-v1      & \href{https://huggingface.co/X-iZhang/libra-v1.0-7b}{\nolinkurl{X-iZhang/libra-v1.0-7b}} \\
LLaVA-Rad     & \href{https://huggingface.co/X-iZhang/libra-llava-rad}{\nolinkurl{X-iZhang/libra-llava-rad}} \\
CheXagent-2   & \href{https://huggingface.co/StanfordAIMI/CheXagent-2-3b-srrg-findings}{\nolinkurl{StanfordAIMI/CheXagent-2-3b-srrg-findings}} \\
RaDialog      & \href{https://huggingface.co/Chantal/RaDialog-interactive-radiology-report-generation}{\nolinkurl{Chantal/RaDialog-interactive-radiology-report-generation}} \\
\bottomrule
\end{tabular}
\end{table*}

% ═══════════════════════════════════════════════════════════════════════
\subsection{Inference Prompts}
\label{sec:prompts}
% ═══════════════════════════════════════════════════════════════════════

Table~\ref{tab:prompts} lists the exact prompt string passed to each model.
An empty entry indicates that the model uses no free-text prompt; instead,
the image is passed directly to the model's native interface.

\begin{table*}[ht]
\centering
\caption{Inference prompt per model (verbatim from \texttt{prompts.py}).}
\label{tab:prompts}
\fontsize{9pt}{11pt}\selectfont
\setlength{\tabcolsep}{4pt}
\begin{tabular}{L{2.5cm} L{8.2cm}}
\toprule
\textbf{Model} & \textbf{Prompt} \\
\midrule
MedGemma
  & \textit{``Describe this X-ray.''} \\
\midrule
MAIRA-2
  & \textit{``Given the current frontal image, provide a description of the findings in the radiology study.''} \\
\midrule
CXRMate
  & \textit{---} \\
\midrule
NV-Reason-CXR
  & \textit{``Provide a comprehensive image analysis, and list all abnormalities.''} \\
\midrule
LIBRA-v1
  & \textit{``Provide a detailed description of the findings in the radiology image.''} \\
\midrule
LLaVA-Rad
  & \textit{``Describe the findings in the radiology image.''} \\
\midrule
CheXagent-2
  & \textit{``Structured Radiology Report Generation for Findings Section.''} \\
\midrule
RaDialog
  & \textit{``You are to act as a radiologist and write the finding section of a chest x-ray radiology report for this X-ray image. Write in the style of a radiologist, write one fluent text without enumeration, be concise and don't provide explanations or reasons.''} \\
\bottomrule
\end{tabular}
\end{table*}

\label{sec:supp_models}

\subsection{Prompt Sensitivity Analysis}
\begin{figure*}[h]
  \centering
  \includegraphics[width=0.8\linewidth]{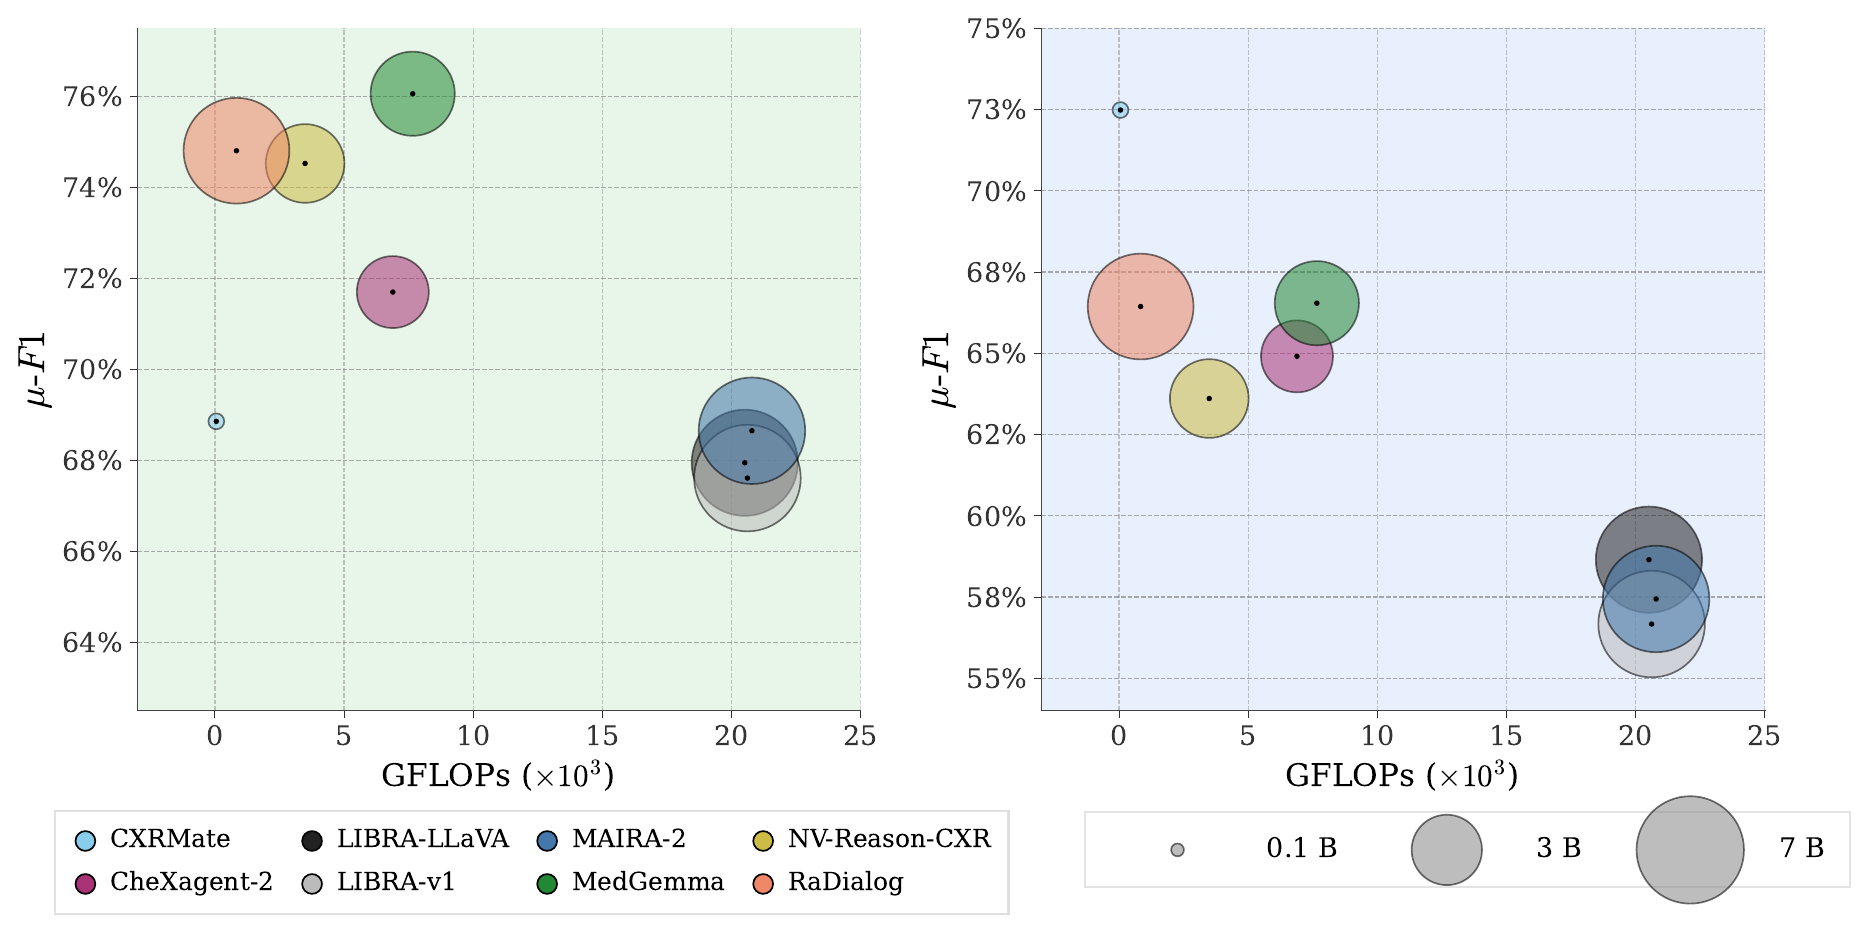}
  \caption{%
  Shortcut scores $\Delta = F_1(\mathrm{RO}_{100}) - F_1(\mathrm{exp}_{100})$
  per model on
  \textcolor{colorMIMIC}{\textbf{MIMIC-CXR}} (left) and
  \textcolor{colorPadChest}{\textbf{PadChest-GR}} (right),
  computed as $\mu\text{-}F_1$ (weighted by class distribution).
  A positive $\Delta$ indicates that the structured occlusion degrades performance
  more than random occlusion.
  \textcolor{colorOCO}{$\Delta_{\mathrm{OCO}}$} reports the effect of
  Object Class Occlusion (full anatomical region masked),
  while \textcolor{colorDOCO}{$\Delta_{\mathrm{DOCO}}$} reports the effect of DOCO.
 }
  \label{fig:flops}
\end{figure*}

\label{sec:prompt_sensitivity}

Since each model is evaluated with its own default prompt (Table~\ref{tab:prompts}), a legitimate concern is whether the benchmark results are sensitive to prompt phrasing rather than to genuine differences in visual grounding.
To address this, we conduct a prompt-matched ablation in which every model receives the same generic instruction (e.g. \textit{``Describe the radiographic findings in this chest X-ray.''}),  while the rest of the \textsc{ShoViR} evaluation pipeline remains unchanged.
CXRMate is excluded from this analysis because it does not accept a textual prompt.

\begin{table}[!h]
\centering
\caption{Prompt sensitivity analysis.
$\Delta_{\text{prompt}} = \mathrm{F1}_{14}^{\text{generic}} - \mathrm{F1}_{14}^{\text{default}}$ (pp) under \textsc{Baseline} (Base.) and \textsc{Full Noise Image} (F.\,Noise).
$\Delta(\Delta_{\mathrm{FN}})$ measures the corresponding change in visual-reliance drop; values near zero indicate prompt robustness.
CXRMate is excluded as it accepts no textual prompt.}
\label{tab:prompt-sensitivity}
\fontsize{7pt}{8pt}\selectfont
\setlength{\tabcolsep}{4pt}
\renewcommand{\arraystretch}{1.10}
\resizebox{1.0\columnwidth}{!}{
\begin{tabular}{L{2.2cm} C{1.0cm} C{1.0cm} C{1.3cm} C{1.0cm} C{1.0cm} C{1.3cm}}
\toprule
& \multicolumn{3}{c}{\textsc{MIMIC-CXR}} & \multicolumn{3}{c}{\textsc{PadChest-GR}} \\
\cmidrule(lr){2-4} \cmidrule(lr){5-7}
\textbf{Model}
  & Base. & F.\,Noise & $\Delta(\Delta_{\mathrm{FN}})$
  & Base. & F.\,Noise & $\Delta(\Delta_{\mathrm{FN}})$ \\
\midrule
RaDialog        & $+0.1$  & $+0.2$   & $-0.1$  & $+5.7$  & $-0.1$   & $+5.8$  \\
CheXagent-2     & $-0.4$  & $-0.9$   & $+0.5$  & $+0.7$  & $+0.3$   & $+0.4$  \\
LLaVA-Rad       & $-1.0$  & $-20.8$  & $+19.8$ & $-3.8$  & $-11.6$  & $+7.8$  \\
Libra-v1        & $-1.3$  & $-4.8$   & $+3.5$  & $-3.0$  & $-2.8$   & $-0.2$  \\
MedGemma        & $+0.2$  & $+2.7$   & $-2.5$  & $-0.8$  & $+0.5$   & $-1.3$  \\
MAIRA-2         & $-1.8$  & $-7.7$   & $+5.9$  & $-1.6$  & $-8.7$   & $+7.1$  \\
NV-Reason-CXR   & $-12.0$ & $-0.3$   & $-11.7$ & $-18.7$ & $-1.6$   & $-17.1$ \\
\bottomrule
\end{tabular}}
\end{table}

Table~\ref{tab:prompt-sensitivity} reports the resulting shift $\Delta_{\text{prompt}} = \mathrm{F1}_{14}^{\text{generic}} - \mathrm{F1}_{14}^{\text{default}}$ under both the \textsc{Baseline} and \textsc{Full Noise Image} conditions, together with $\Delta(\Delta_{\mathrm{FN}})$, which measures how the visual-reliance drop (Eq.~2 in the main paper) changes when switching from the default to the generic prompt.
Values of $\Delta(\Delta_{\mathrm{FN}})$ near zero indicate that the relative ordering of visual reliance is preserved regardless of prompt choice.

Two findings emerge from this analysis.
First, prompt substitution has a limited effect on clean-image performance: under \textsc{Baseline}, six of seven models remain within $\pm 6$ percentage points of their default-prompt scores on both datasets.
The sole exception is NV-Reason-CXR, which drops by $-12.0$\,pp on MIMIC-CXR and $-18.7$\,pp on PadChest-GR; this is expected, as its chain-of-thought reasoning template is tightly coupled to the training prompt, and replacing it disrupts the model's structured output format.

Second, the visual-reliance ranking is largely preserved.
Five of seven models show $|\Delta(\Delta_{\mathrm{FN}})| \leq 6$\,pp, confirming that the gap between \textsc{Baseline} and \textsc{Full Noise Image} performance is stable across prompt formulations.
The two outliers admit straightforward explanations.
For NV-Reason-CXR, the large negative $\Delta(\Delta_{\mathrm{FN}})$ ($-11.7$ on MIMIC-CXR, $-17.1$ on PadChest-GR) is driven entirely by the \textsc{Baseline} collapse described above; its \textsc{Full Noise Image} scores shift by only $-0.3$ and $-1.6$\,pp, respectively, meaning that the model's behavior under noise is essentially unchanged.
For LLaVA-Rad, the positive $\Delta(\Delta_{\mathrm{FN}})$ ($+19.8$ on MIMIC-CXR, $+7.8$ on PadChest-GR) indicates that the generic prompt \emph{amplifies} the model's sensitivity to noise removal, widening the gap between clean and corrupted inputs.
This is consistent with LLaVA-Rad's default prompt providing implicit cues that partially compensate for missing visual content, an effect that vanishes under the generic formulation.

Finally, the disease-level shortcut metrics reported in Section~4.3 of the main paper are inherently invariant to prompt choice: both $\Delta_{\mathrm{OCO}}$ and $\Delta_{\mathrm{DOCO}}$ are computed as pairwise differences between occlusion conditions evaluated under the same prompt, so any prompt-induced offset cancels out.

% ═══════════════════════════════════════════════════════════════════════
\subsection{Decoding Hyperparameters}

\label{sec:decoding}

Table~\ref{tab:decoding} lists the decoding configuration used for each model.
We adopt the default settings provided by the original authors or official repositories whenever available, adjusting only the maximum number of new tokens (MNT) when necessary to ensure complete report generation.
Most models rely on greedy decoding (beam width of one), while CXRMate employs beam search and LIBRA-v1 and LLaVA-Rad use sampling with a low temperature.
Where a parameter is not applicable (\textit{e.g.}, temperature under greedy decoding), a dash is shown.

\begin{table}[!h]
\centering
\caption{Decoding hyperparameters per model. MNT = maximum new tokens.}
\label{tab:decoding}
\fontsize{9pt}{11pt}\selectfont
\resizebox{1.0\columnwidth}{!}{
\begin{tabular}{L{2.2cm} C{1.2cm} C{1.0cm} C{1.0cm} C{1.0cm} C{1.0cm}}
\toprule
\textbf{Model} &
\textbf{MNT} &
\textbf{Beams} &
\textbf{Temp.} &
\textbf{Top-$k$} &
\textbf{Top-$p$} \\
\midrule
MedGemma        & 450  & 1 & 1.0            & 50 & 1.0 \\
MAIRA-2         & 450  & 1 & 1.0            & 50 & 1.0 \\
CXRMate$^{a}$   & 128  & 4 & 1.0            & 50 & 1.0 \\
NV-Reason-CXR   & 2048 & 1 & $10^{-6}$      & 50 & 1.0 \\
LIBRA-v1        & 300  & 1 & 0.20           & 50 & --- \\
LLaVA-Rad       & 1024 & 5 & 0.20           & 50 & --- \\
CheXagent-2     & 512  & 1 & 1.0            & 50 & 1.0 \\
RaDialog        & 300  & 1 & 1.0            & 50 & 1.0 \\
\bottomrule
\multicolumn{6}{l}{\scriptsize $^{a}$~CXRMate uses beam search with \texttt{bad\_words\_ids} to suppress non-findings tokens.}
\end{tabular}
}
\end{table}
% ═══════════════════════════════════════════════════════════════════════

%═══════════════════════════════════════════════════════════════════════
\subsection{Computational Cost}

\label{sec:common}
Figure~\ref{fig:flops} jointly visualises diagnostic quality ($\mu$-$F_1$) and inference cost (GFLOPs per image, bubble area $\propto$ model size in parameters). 
The models span three orders of magnitude in compute: CXRMate-RRG24 (0.15 B parameters, 54.6 GFLOPs) sits at the far left of both panels, delivering competitive performance at a fraction of the cost of larger counterparts. 
The three 7 Billions parameters models: MAIRA-2, LIBRA-v1, and LLaVA-Rad at the high-compute end ($\approx$ 20,500–20,800 GFLOPs), yet do not uniformly dominate in $\mu$-$F_1$. 
RaDialog is a notable outlier: despite its 6.8 B parameter count, has the lowest GFLOPs cost over the large-model group. 
Mid-range models (NV-Reason-CXR, CheXagent-2, MedGemma; 3–4 B parameters, 3,500–7,700 GFLOPs) occupy an intermediate efficiency regime. 
Across both datasets, the absence of a clear positive trend between GFLOPs and $\mu$-$F_1$ indicates that raw model scale is not the primary driver of radiology report quality in this benchmark; architectural choices-particularly the vision encoder and domain pre-training-appear more decisive than parameter count alone.

% ═══════════════════════════════════════════════════════════════════════
\section{Experimental Settings}
\label{sec:common}
% ═══════════════════════════════════════════════════════════════════════

All experiments were conducted on the \texttt{Anonymous} cluster using 8 NVIDIA A40 GPUs (48\,GB VRAM each), managed via SLURM. Models were run in dedicated virtual environments to handle conflicting dependencies, using PyTorch 2.1+ with bfloat16 precision throughout. 

\begin{table}[h]
\centering
\caption{Common settings shared across all model experiments.}
\label{tab:common}
\small
\resizebox{1.1\columnwidth}{!}{
\begin{tabular}{L{4.2cm} L{7.8cm}}
\toprule
\textbf{Setting} & \textbf{Value} \\
\midrule
Dataset            & PadChest-GR, MIMIC-CXR \\
Hardware           & 8$\times$ NVIDIA A40 (48\,GB VRAM each) \\
Scheduler          & SLURM \\
Python version     & 3.11.5 \\
Framework          & PyTorch 2.1$+$, HuggingFace Transformers 4.40$+$ \\
Precision          & bfloat16 \\
Output format      & JSONL per model/experiment \\
Occlusion levels   & $p \in \{0, 20, 40, 60, 80, 100\}\%$ \\
Evaluation metrics & BLEU-1/2/4, ROUGE-L, RadGraph-F1,
                     CheXBERT per-class F1, $\mu$-F1, GREEN \\
\bottomrule
\end{tabular}
}
\end{table}

% ---- Bibliography ----
%
% BibTeX users should specify bibliography style 'splncs04'.
% References will then be sorted and formatted in the correct style.
%
\bibliographystyle{splncs04}
\bibliography{biblio}
\end{document}
